# Supplementary material for: DoseGNN: Improving the Performance of Deep Learning Models in Adaptive Dose-Volume Histogram Prediction through Graph Neural Networks
Source: arXiv:2402.01076 source file (2024-02-02)
Supplement: Supplementary file 1 [file 8_supplementary.tex]

\section{Representation Learning Tasks on Gene Networks and Other Graph Benchmarks}
\label{sec:appenA}

In the natural world, genes don’t operate independently and always function as part of a set of genes. Hence, they can be regulated as the graph modality based on reported genetic interactions that underlie phenotypes in a variety of bioinformatical systems. Then, various computational tasks on gene networks (graphs) are proposed in recent bioinformatics to numerically analyze contribution of genes to complex disease in humans. In this work, we take two long-standing challenging tasks in bioinformatics, Alzheimer’s disease (AD) classification and cancer subtype classification, as example, and introduces corresponding gene-network datasets. Here we compare the these gene network datasets against popular graph benchmark datasets to illustrate challenges of graph representation learning over gene networks. 

\begin{table*}[th]
%\vskip -0.22in
%\vskip -0.1in
\centering
\resizebox{0.8\textwidth}{!}{
\begin{tabular}{lccccc}
\toprule
Dataset & Ave. $\#$ nodes & Ave. $\#$ edges  & $\#$ Tasks & Task Type & Metric \\ 
\midrule
Mayo &  3000  & 60000 & 2 & Classification & Accuracy $\&$ F1\\
RosMap & 3000 & 60000 & 2 & Classification & Accuracy $\&$ F1\\
Cancer Subtype & 3800 & 48000 & 7  & Classification & Accuracy $\&$ F1 \\
\midrule
NA & 8  & 12 & 1 & Regression & RMSE $\&$ Pearson'r \\
BN & 10  & 15 & 1 & Regression & RMSE $\&$ Pearson'r \\
ogbg-molhiv & 26 & 55 &  2 & Classification & ROC-AUC \\
ZINC & 23 &  50 & 1 & Regression & MAE \\
D$\&$D & 284 & 1431 & 2 & Classification & Accuracy \\
MUTAG & 18 & 39 & 2 & Classification & Accuracy \\
PROTEINS & 39 & 146 & 2 & Classification & Accuracy \\
PTC-MR & 14 & 29 & 2 & Classification & Accuracy \\
ENZYMES & 33 & 124 & 6 & Classification & Accuracy \\

%Life Span & graph regression & 1 & Pearson'r $\&$ rmse \\
\bottomrule
\end{tabular}
}
\caption{Comparison of gene networks and graphs in popular benchmark datasets}
\label{table:dataset}
\end{table*}

Table ~\ref{table:dataset} presents preliminary results. Compared to graphs in popular benchmarks, gene networks always contain significantly large number of nodes (denoted as $n$) as well as the number of edges (denoted as $m$), which limits the applicability of popular expressive GNNs due to the complexity consideration. For subgraph-based GNNs like NGNN ~\citep{zhang2021nested}, the space complexity grows exponentially as the average node degree $\frac{m}{n}$ increases. For high-order GNNs, such as k-WL ~\citep{morris2019weisfeiler} and k-FWL ~\citep{grohe2021logic}, that mimic the high-order WL algorithms, the stable colourings/representations can be computed in $\mathcal{O}(k^2 n^{k+1}\log n)$ with a space complexity of $\mathcal{O}(n^{k})$. Consequently, it is hard to apply these methods to gene network representation learning.

\section{More Discussion of GC-GNN and UGC-GNN}
\label{sec:appenB}

In this section, we provide more discussion of GC-GNN. 

\begin{itemize}
    \item \textbf{Part 1:} Limitations of GC-GNN and UGC-GNN.
    \item \textbf{Part 2:} The complexity of GC-GNN and UGC-GNN. 
\end{itemize}

\paragraph{Part 1 (Table ~\ref{table:molecular})} One significant limitation of GC-GNN and UGC-GNN is that the (universal) graph canonization fail to consider the heterogeneity among edges. In addition, GC-GNN is also not guaranteed to be suitable for all graph learning tasks. Here we empirically test GC-GNN on moleculr datasets, ogbg-molhiv and ogbg-molpcba, in Open Graph Benchmark~\citep{hu2020open}. Table ~\ref{table:molecular} provides empirical results. As we can see, though in most cases GC-GNN still improve the performance over backbone GNNs, the improvement is not significant as TU datasets and GC-GNN can not achieve the SOTA performance. In some cases, the graph canonization even causes a performance decrement over the GNN backbone. The performance decrease might be explained by the utilization of atom encoders in ogbg-molhiv, which generate learnt embedding for more efficient representation learning, while these learnt nde embeddings are not suitable for graph canonization algorithms. Then the performance improvement from distinguishing more graph structures can not overwhelm the decrease from deteriorated mode stability.

\begin{table}[ht]
\centering
\resizebox{0.56\textwidth}{!}{
\begin{tabular}{lcc}
\toprule
&  ogbg-molhiv ( AUC $\uparrow$) & ogbg-molpcba (AP $\uparrow$ ) \\
\midrule
GCN (backbone) & 0.7501 $\pm$ 0.0140 & 0.2422 $\pm$ 0.0034 \\
\textbf{GN-GCN} & \color{red}0.7609 $\pm$ \color{red}0.0158 & \color{red} 0.2510 $\pm$ 0.0047   \\
\midrule
GIN (backbone) & 0.7744 $\pm$ 0.0098 & 0.2703 $\pm$ 0.0023   \\
\textbf{GN-GIN} & \color{blue}0.7307 $\pm$ \color{blue}0.0198   & \color{red} 0.2761 $\pm$ 0.0043 \\ 
\bottomrule
\end{tabular}
}
\caption{Empirical results on molecular datasets. Performance \color{red} increment \color{black}and  \color{blue} decrement  \color{black} are visualized as colors.}
\label{table:molecular}
\end{table}

\paragraph{Part 2} The main concern of complexity comes from the graph canonization algorithms. As we discussed in the main paper (section 1.1, other related works), although graph canonization is a well-know NP-complete problem, practical canonization tools such as Nauty~\citep{mckay2014practical} and Bliss ~\citep{junttila2012bliss}, can effectively solve the problem in practice with an average time complexity of $\mathcal{O}(n)$. The process of computing the canonical forms of graphs can be implemented in the graph pre-process phase and we only need to perform practical graph canonization tools once for each graph.
Furthermore, as the output discrete colouring $\{\rho(v_1| G), \rho(v_2| G) ... \rho(v_n| G)\}$ of graph canonization are used as positional encodings of nodes, the additional space complexity is also $\mathcal{O}(n)$. Hence, compared to dominant expressive GNNs like subgraph-based GNNs and high-order GNNs, GC-GNN (UGC-GNN) is much more efficient with a significant low space and computation cost. For instance, on ogbg-molhiv, GC-GNN (GIN) takes $39$ seconds per epoch, while Nested GIN takes $168$ seconds. 

\section{Proof of Lemma~\ref{lemma:2_4} and Lemma~\ref{lemma:2_3}}
\label{sec:appenC}

We first prove Lemma~\ref{lemma:2_4}. Since discrete colouring $\{\rho(v_1|G), \rho(v_2|G), ..., \rho(v_n|G)\}$ generated by graph canonization provides a unique way to label nodes for graphs in the same isomorphic group $ISO(G)$, then the isomorphism of two graphs can be determined by checking whether the node pairs of the same labels share the same edge relation. When the graph convolution layers on GNN $g$ are injective, it can injectively map the pair of a node and the set of its' neighboring nodes.  then if two graphs get different sets of learnt node embeddings by the GNN $g$,  there must exists at least one pair of node label and the set of its' neighboring nodes' labels are different. Then, these two graphs are not isomorphic. On the other hand, when two graphs are not isomorphic, there must be at least one pair of nodes with the same labels, while the pair of nodes are connected in one graph yet disconnected in another graph. Then the graph convolution layer will output different embeddings for each node in the node pair.

Next, we prove Lemma~\ref{lemma:2_3} to support theoretical results about the stability of GNNs and GC-GNNs. Before proving our lemma, we first introduce some necessary preliminaries that we will later use in the proofs.

\paragraph{Preliminary 1: Decomposition of message passing layer of GNNs} The message passing scheme adopted in popular GNNs iteratively updates a node’s representation/embedding according to the multiset of its neighbors’ representations/embeddings and its current representation/embedding. Let $h^{t}_{v}$ denotes the representation of $v$ in layer $t$, the massage passing scheme is given by:
\begin{align*}
     h^{t+1}_v & = \mathcal{M}(h^{t}_{v}, \{h^{t}_{u} | (u,v) \in E \}) \\
     & = \mathcal{U}(h^{t}_{v}, \mathcal{A} (\{h^{t}_{u} | (u,v) \in E\})) 
\end{align*}
Here, $\mathcal{A}$ is an aggregation function on the multiset $S =  \{h^{t}_{u} | (u,v) \in E \})$ and $\mathcal{U}$ is an update function. 

\begin{defi}
\label{defi:c_1}
    A function $f$ is claimed as a L-stable multiset function if 1) $\sum_{h \in S} f(h)$ is unique for each multiset $S$ of bounded size; and 2) for any two multisets $S_1$ and $S_2$,  $|| \sum_{h \in S_1} f(h) -$ $\sum_{h^{'} \in S_2} f(h^{'}) ||$ $\leq L \times d_S(S_1, S_2)$, where $d_S(S_1, S_2) = |S_1| + |S_2| - |S_1 \cap S_2|$.  
\end{defi}
The L-stable multiset function $f$ provides a unique mapping between the multiset space and representation space, while distance between multisets in the representation space are bounded through the constant multplier L.  

\begin{coro}
    \label{coro:c_1}
    Assume that input feature space $\mathbb{H}$ is countable. Any message passing function $\mathcal{M}$ over pairs $(h, S)$, where $h \in \mathbb{H}$ and $S \subset \mathbb{H}$, can be decomposed as $\mathcal{M}(h,S) = \phi((1+ \epsilon) f(h) + \sum_{h^{'} \in S} f(h^{'}))$ for some L-stable multiset function $f$, some function $\phi$ and infinitely many choices of $\epsilon$.
\end{coro}

This corollary ~\ref{coro:c_1} can be obtained by following the Lemma 5 and Corollary 6 in \cite{xu2018how}. Basically, since the space $\mathbb{H}$ is countable, we can always get a mapping $Z: \mathbb{H} \to \mathbb{N} $ from $h \in \mathbb{H}$ to natural numbers. As $S$ are bounded multiset, there always exists an upper bound $B$ of their cardinality such that $|S| < B$ for any $S$. Hence, the example function $f(h) = B^{-Z(h)}$ satisfies both the uniqueness condition as well as the inequality condition in Definition ~\ref{defi:c_1} where the constant $L = \frac{1}{B}$.

\paragraph{Preliminary 2: Graph canonization and individualization-and-refinement paradigm}
Here we provide an extended discussion on the graph canonization and individualization-refinement paradigm. To address the complex graph isomorphism/ graph canonization problem, practical graph canonization tools resort to the individualization-and-refinement paradigm, where the color refinement and individualization steps are iteratively performed to get a discrete colouring. 
\begin{itemize}
    \item 1. Color refinement step: The color refinement algorithm aims to recolor nodes in a graph by similarity. The algorithm starts with some initial node colors, then the algorithm updates node's color round by round, and in each round, two nodes with the same color will get different new color if the multiset of neighboring colors are different. This process continues until an equitable colouring is obtained such that the node colors will not change even if another color refinement round happens.
    \item 2. Individualization step: When a stable colouring generated by the color refinement step is discrete, then returns a order of nodes in the canonical form. However, in many cases, the stable colouring are not discrete. Then the individualization step selects a node in a color class with more than one node and assigns a new (unseen) color to the node. Then the color refinement step is implemented again.
\end{itemize}

Specifically, in the color refinement step, the new colors are obtained by lexicographically sorting the pair of node current color and it's multiset of neighboring colors. Hence, the new order of new node colors always follows that of the previous colors. That is, at round $t$, if two nodes $v$, $u$ have different colors $c^{t}(u)$ and $c^{t}(v)$ such that $c^{t}(u) < c^{t}(v)$, then after one round of color refinement, the new colors of these two nodes have $c^{t+1}(u) < c^{t+1}(v)$.

Above individualization-refinement paradigm in practical graph canonization tools provide a solution to obtain a discrete coloring, yet not in a canonical way. That is, generated discrete coloring is not guaranteed to be the same for graphs in the same isomorphic class.  To fix this, practical tools usually branch on all nodes of the same color in the individualization step and individualizes one node in each branch. Then a tree of colouring can be obtained such that each leaf of the tree is a discrete coloring of the input grpah $G$. Then the final discrete colouring is selected, for example, as the leaf with the lexicographically minimal string that consists of the rows of the adjacency matrix according to the discrete colouring (i.e. node orders). More details can be found in \cite{mckay2014practical}.

\paragraph{\textit{Proof.} (Part one: A GNN model $g$ is stable under $X$)} Here, we assume the function $\phi$ in the decomposition of message passing layer of GNNs is K-Lipschitz. A function $\phi: (X, d_x) \to (Y, d_y)$ between two metric spaces is K-Lipschitz if $d_y(\phi(x_1), \phi(x_2)) \leq Kd_x(x_1, x_2)$ for any $x_1, x_2 \in X$, where K is a constant. 

\begin{coro}
    \label{coro:c_2}
    MLPs are K-Lipschitz.
\end{coro}

In popular message passing GNNs, $\phi$ is always modeled by a MLP. Hence, we need to prove corollary ~\ref{coro:c_2} to use the K-Lipschitz assumption. For each MLP layer that characterized by the trainable parameter tensors $W_i$ and $b_i$ (bias), it can be represented as $\sigma(W_i x + b_i)$, where $\sigma$ is the activation function. Then we have $|| \sigma(W_i x_1 + b_i) - \sigma(W_i x_2 + b_i)|| = || \frac{\partial \sigma}{\partial x} W_i (x_1 - x_2)||$. Since the activation function $\sigma$ usually takes ReLU/sigmoid/tanh, it's straightforward that $|| \frac{\partial \sigma}{\partial x} ||$ is bounded by a constant $K_1$. Then we get $|| \frac{\partial \sigma}{\partial x} W_i (x_1 - x_2)|| \leq K_1 || W_i ||_2 ||x_1 - x_2||$, where $K_1 || W_i ||_2$ is a constant independent of $x_1$ and $x_2$. Hence, we show that MLPs are K-Lipschitz.

Next, let's prove the theoretical result. Without loss of generality, we assume that the GNN contains a single message passing layer. For any two graphs $G^{(1)} = (A^{(1)}, X^{(1)})$ and $G^{(2)} = (A^{(2)}, X^{(2)})$, let $\pi^{*} \in \Pi(n)$ denotes the optimal permutation operation that best aligns the $G_1$ and $G_2$, and $P^{*}$ is the corresponding permutation matrix. Then we have,

\scriptsize
\begin{align}
    &||g(A^{(1)}, X^{(1)}) - g(A^{(2)}, X^{(2)})||   \notag \\
    = &||\sum_{v \in G^{(1)}}\phi((1+ \epsilon)f(X^{(1)}_v) + \sum_{v^{'} \in \mathcal{N}(v|G^{(1)})} f(X^{(1)}_{v^{'}})) -  \sum_{u \in G^{(2)}}\phi((1+ \epsilon)f(X^{(2)}_u) + \sum_{u^{'} \in \mathcal{N}(u|G^{(2)})} f(X^{(2)}_{u^{'}}))|| \\
     \leq & \sum_{v \in G^{(1)}} ||\phi((1+ \epsilon)f(X^{(1)}_v) + \sum_{v^{'} \in \mathcal{N}(v|G^{(1)})} f(X^{(1)}_{v^{'}})) -  \phi((1+ \epsilon)f(X^{(2)}_{\pi^{*}(v)}) + \sum_{u^{'} \in \mathcal{N}(\pi^{*}(v)|G^{(2)})}f(X^{(2)}_{u^{'}}))|| \\
     \leq & K \sum_{v \in G^{(1)}} ||(1+ \epsilon)f(X^{(1)}_v) + \sum_{v^{'} \in \mathcal{N}(v|G^{(1)})} f(X^{(1)}_{v^{'}}) -  (1+ \epsilon)f(X^{(2)}_{\pi^{*}(v)}) - \sum_{u^{'} \in \mathcal{N}(\pi^{*}(v)|G^{(2)})}f(X^{(2)}_{u^{'}})|| \\
     \leq & K(1+ \epsilon) \sum_{v \in G^{(1)}} ||f(X^{(1)}_v)-f(X^{(2)}_{\pi^{*}(v)})|| + K\sum_{v \in G^{(1)}} || \sum_{v^{'} \in \mathcal{N}(v|G^{(1)})} f(X^{(1)}_{v^{'}}) 
 - \sum_{u^{'} \in \mathcal{N}(\pi^{*}(v)|G^{(2)})}f(X^{(2)}_{u^{'}})|| \\
 \leq & K\times L \times (1+ \epsilon) (\sum_{v} X^{(1)}_{v} \neq X^{(2)}_{\pi^{*}(v)}) + K \times L \times d_S (\mathcal{N}(v|G^{(1)}), u^{'} \in \mathcal{N}(\pi^{*}(v)|G^{(2)})) \\
 \leq & K\times L \times (1+ \epsilon) d(G^{(1)}, G^{(2)})
\end{align}

\normalsize
Here, we use the K-Lipschitz property in the step (4), and use the property of L-stable multiset function in step (6). Furthermore, $\mathcal{N}(v|G^{(1)})$ denotes the set of neighboring nodes of $v$ in $G^{(1)}$, and can be characterized by the $v$th row of adjacency matrix $A^{(1)}$. $\mathcal{N}(\pi^{*}(v)|G^{(2)})$ denotes the set of neighboring nodes of $v$'s image in $G^{2}$, and can be characterized by the $v$th row of adjacency matrix $P^{*}A^{(2)}P^{*T}$. Hence, we show that GNN $g$ is stable under $X$ with a constant $C$ of $K\times L \times (1+ \epsilon)$.

\paragraph{\textit{Proof.} (Part two: A GNN model $g$ is not stable under $X \oplus P$)}
Here we provide a counter example. Let $G^{(1)}$ be a graph of $n$  nodes such that 1) there is no node symmetry in the graph; 2) the node $v_n$ has an initial color (integer feature) that is strictly larger than the colors of other nodes. Then, we obtain a graph $G^{(2)}$ by changing the initial color of node $v_n$ in $G^{(1)}$ to another color which is strictly smaller than the colors of other nodes. Then, we know that there is no node symmetry in the graph $G^{(2)}$, either. Furthermore, it's straightforward that the best graph matching $\pi^{*} \in \Pi(n)$ between $G^{(1)}$ and $G^{(2)}$ is $\pi(i) = i$ for $\forall i = 1,2,...n$ and the corresponding permutation matrix $P^{*} = I$ is an identity matrix.

Since there is no node symmetry in $G^{(1)}$ and $G^{(2)}$, the color refinement step in graph normalization tools will generate discrete colourings for $G^{(1)}$ and $G^{(2)}$. Let $\{\rho(v_1|G^{(1)}), \rho(v_2|G^{(1)}), ..., \rho(v_n|G^{(1)})\}$ and $\{\rho(v_1|G^{(2)}), \rho(v_2|G^{(2)}), ..., \rho(v_n|G^{(2)}\}$ denote the corresponding discrete colourings. As we discussed in preliminary 2, the output discrete colouring from color refinement will keep the order of initial colors. Hence, we know that $\rho(v_n|G^{(1)})=n$, $\rho(v_n|G^{(2)})=1$ and $\rho(v_i|G^{(1)})=\rho(v_i|G^{(2)}) + 1$ for $i = 1,2, ... n-1$. Thus, we get $\rho(v_i|G^{(1)}) \neq \rho(v_i|G^{(2)})$ for $i = 1,2,..., n$, indicating that $P^{(1)}_{v} \neq P^{(2)}_{v}$ for $\forall v$. Thus, we have,

\begin{align}
&||g(A^{(1)}, X^{(1)}) - g(A^{(2)}, X^{(2)})||   \notag \\
\geq & || \sum_{v \in G^{(1)}} (1+ \epsilon)(f(X^{(1)}_v+P^{(1)}_v) - f(X^{(2)}_v+P^{(2)}_v))|| \\
\geq & (1+ \epsilon) \times |G^{(1)}| \times \frac{1}{B} \\
\geq & 1 = d(G^{(1)}, G^{(2)})
\end{align}

Since the function $f$ is defined on the multiset whose cardinality is bounded by the overall graph size $n$, we get $B \leq |G^{(1)}|$.

\section{Proof of Theorem~\ref{theo:3_2}}
\label{sec:appenD}
\textit{Proof.} Following the proof of Lemma \ref{lemma:2_3}, we consider the same decomposition scheme $\mathcal{M}(h,S) = \phi((1+ \epsilon) f(h) + \sum_{h^{'} \in S} f(h^{'}))$ of the message passing layer, yet the input space is $X \oplus P$ (where $P$ is the 2-dimensional tensor of one-hot encodings of discrete colouring generated by universal graph normalization), instead of the input feature $X$. 

Then, let's consider any pairs $\mathcal{N}(v|G^{(1)}))$ and $\mathcal{N}(\pi^{*}(v)|G^{(2)}))$. Since the discrete colouring in any common subgraph $G^{'}$ of $G^{(1)}$ and $G^{(2)}$ are identical, %Then, let's consider any pairs of $(v, \mathcal{N}(v|G^{(1)}))$ in $G^{(1)}$ and $(\pi^{*}(v), \mathcal{N}(\pi^{*}(v)|G^{(2)}))$ in $G^{(2)}$. If we have $P^{(1)}_{v} = P^{(2)}_{\pi^{*}(v)}$, then we know that there exists a common subgraph $G^{'}$ of $G^{(1)}$ and $G^{(2)}$ that contains node $v \in G^{(1)}$ ($\pi^{*}(v) \in G^{(2)}$). As such, if any $v^{'} \in \mathcal{N}(v|G^{(1)})$ and $u^{'} \in \mathcal{N}(\pi^{*}(v)|G^{(2)})$ such that $X^{(1)}_{v^{'}} = X^{(2)}_{u^{'}}$, then we have $P^{(1)}_{v^{'}} = P^{(2)}_{u^{'}}$, as $v^{'}$ ( $u^{'}$) can be obtained in $G^{'}$ in $G^{(1)}$ (in $G^{(2)}$) to formulate a larger common subgraph. Thus, 
the number of same items in multisets $\{X^{(1)}_{v^{'}}| v^{'} \in \mathcal{N}(v|G^{(1)}) \}$ and $\{X^{(2)}_{u^{'}}| u^{'} \in \mathcal{N}(\pi^{*}(v)|G^{(2)}) \}$ will not change if we replace $X^{(1)}_{v^{'}}$ with $X^{(1)}_{v^{'}} + P^{(1)}_{v^{'}}$, and $X^{(2)}_{u^{'}}$ with $X^{(2)}_{u^{'}} + P^{(2)}_{u^{'}}$. Then we get, 
\small
\begin{align}
    & \sum_{v^{'} \in \mathcal{N}(v|G^{(1)})} f(X^{(1)}_{v^{'}}+ P^{(1)}_{v^{'}}) - \sum_{u^{'} \in \mathcal{N}(\pi^{*}(v)|G^{(2)})}f(X^{(2)}_{u^{'}} + P^{(2)}_{u^{'}}) \notag \\
    = & \sum_{v^{'} \in \mathcal{N}(v|G^{(1)})} f(X^{(1)}_{v^{'}}) - \sum_{u^{'} \in \mathcal{N}(\pi^{*}(v)|G^{(2)})}f(X^{(2)}_{u^{'}})
\end{align}

\normalsize
Thus, we have 

\small
\begin{align}
    &||g(A^{(1)}, X^{(1)}) - g(A^{(2)}, X^{(2)})||   \notag \\
    = & ||\sum_{v \in G^{(1)}}\phi((1+ \epsilon)f(X^{(1)}_v + P^{(1)}_v) + \sum_{v^{'} \in \mathcal{N}(v|G^{(1)})} f(X^{(1)}_{v^{'}}+P^{(1)}_{v^{'}})) \notag \\ 
    & -  \sum_{u \in G^{(2)}}\phi((1+ \epsilon)f(X^{(2)}_u + P^{(2)}_u) + \sum_{u^{'} \in \mathcal{N}(u|G^{(2)})} f(X^{(2)}_{u^{'}} + P^{(2)}_{u^{'}}))|| \\  
    \leq & K \sum_{v \in G^{(1)}} ||(1+ \epsilon)f(X^{(1)}_v + P^{(1)}_v) + \sum_{v^{'} \in \mathcal{N}(v|G^{(1)})} f(X^{(1)}_{v^{'}} + P^{(1)}_{v^{'}}) \notag \\
    &-  (1+ \epsilon)f(X^{(2)}_{\pi^{*}(v)} + P^{(2)}_{\pi^{*}(v)}) - \sum_{u^{'} \in \mathcal{N}(\pi^{*}(v)|G^{(2)})}f(X^{(2)}_{u^{'}} + P^{(2)}_{u^{'}})|| \\
    \leq &  K (1 + \epsilon) \sum_{v \in G^{(1)}} ||f(X^{(1)}_v + P^{(1)}_v) -  f(X^{(2)}_{\pi^{*}(v)} + P^{(2)}_{\pi^{*}(v)})|| \notag \\
    & + K \sum_{v \in G^{(1)}} ||\sum_{v^{'} \in \mathcal{N}(v|G^{(1)})} f(X^{(1)}_{v^{'}}+ P^{(1)}_{v^{'}}) - \sum_{u^{'} \in \mathcal{N}(\pi^{*}(v)|G^{(2)})}f(X^{(2)}_{u^{'}} + P^{(2)}_{u^{'}}) || \\
    = &  K (1 + \epsilon) \sum_{v \in G^{(1)}} ||f(X^{(1)}_v + P^{(1)}_v) -  f(X^{(2)}_{\pi^{*}(v)} + P^{(2)}_{\pi^{*}(v)})|| \notag \\
    & + K \sum_{v \in G^{(1)}} ||\sum_{v^{'} \in \mathcal{N}(v|G^{(1)})} f(X^{(1)}_{v^{'}}) - \sum_{u^{'} \in \mathcal{N}(\pi^{*}(v)|G^{(2)})}f(X^{(2)}_{u^{'}}) || \\
    \leq & K\times L \times (1+ \epsilon) d(G^{(1)}, G^{(2)})
\end{align}

\normalsize
where we use the equation (11) in the step (14) to get step (15).

\section{Proof of Lemma~\ref{lemma:3_4}}
\label{sec:appenE}
\textit{Proof.} Since the function $l(v|\mathbb{G}): V \to \mathbb{N}$ is an injective function, it can distinguish nodes in each graph according to $l(v|\mathbb{G})$. Furthermore, since for $\forall$ $v_1, u_1 \in G_1$, $v_2, u_2 \in G_2$, $G_1, G_2 \in \mathbb{G}$ such that $l(v_1|\mathbb{G}) = l(v_2|\mathbb{G})$ and $l(u_1|\mathbb{G}) = l(u_2|\mathbb{G})$, we have $(v_1, u_i) \in E_1$ $\leftrightarrow$ $(v_2, u_2) \in E_2$, we know that the connectivity between node pairs $(v,u)$ of the same label pairs $(l(v|\mathbb{G}), l(u|\mathbb{G}))$ is shared among all graphs. Let N be the total number of all potential different labels $l(v|\mathcal{G})$, then we can expand each graph to a larger graph of size N, where each node $v$ has an order/position of $l(v|\mathcal{G})$, and rest positions are padded by dummy nodes that is not connected with any other nodes. Then, any common subgraph $G^{'}$ of $G_1$ and $G_2$, is also a common subgraph of their converted larger graphs, and it is obivous that the orders of nodes in each common subgraph of these generated larger graphs are identical.

\section{Proof of Lemma~\ref{lemma:3_5}}
\label{sec:appenF}
\textit{Proof.} Let $G = (A,X)$ be an arbitrary graph of size $n$, and $\forall P \in \Pi(n)$ where $\Pi(n)$ is the permutation group. $\{l(v_1| \mathbb{G}), l(v_2| \mathbb{G}) ... l(v_n| \mathbb{G})\}$ is the discrete colouring of $G$ generated by the universal graph canonization. The discrete colouring is invariant to the permutation operation $P$ as graphs from the same isomorphic class has the same canonical form (so as the same output discrete colouring from universal graph canonization). Here, we use $L$ to denote a $2$-dimension tensor of one-hot features of this discrete colouring. Then, let $G^{'} = (PAP^{T}, PX)$ ($G^{'}$ is isomorphic to $G$), then, the corresponding discrete colouring tensor is $PL$. Let $\mathcal{M}$ be a stack of message passing layers, then we have $P\mathcal{M}(A,X) = \mathcal{M}(PAP^{T}, PX)$ for $\forall X, A$. Let $\mathcal{R}$ denote the readout function of UNGNN, that is $\mathcal{R}(\{h_{v} | v \in V\}) = \sum_{v \in V} W_{l(v| \mathbb{G})}h_{v}$, then $\mathcal{R}$ is invariant to the order of $\{h_{v} | v \in V\}$ as the corresponding weight matrix $W_{l(v| \mathbb{G})}$ is solely decided by node's discrete color $l(v| \mathbb{G})$. Hence, UNGNN $g$ is a composition of functions $\mathcal{R}$ and $\mathcal{M}$, then we get:
\begin{align*}
    g(PAP^{T}, PX) &= \mathcal{R}(\mathcal{M}(PAP^{T}, PX+PL)) \\
    &= \mathcal{R}(\mathcal{M}(PAP^{T}, P(X+L))) \\
    &= \mathcal{R}(P\mathcal{M}(A, X+L)) \\
    &= \mathcal{R}(\mathcal{M}(A, X+L)) = g(A,X)
\end{align*}

\section{More Ablation Results}
\label{sec:appenG}

\begin{table*}[h]
%\vskip -0.1in
\begin{center}
%\Large
\resizebox{0.99\textwidth}{!}{
\begin{tabular}{lcccccccc}
\toprule
& \multicolumn{2}{c}{Mayo} & & \multicolumn{2}{c}{RosMap} & &  \multicolumn{2}{c}{Cancer Subtype} \\
\cmidrule(r){2-3}  \cmidrule(r){5-6} \cmidrule(r){8-9}
Methods  & Accuracy $\uparrow$ & F1 score $\uparrow$ & & Accuracy $\uparrow$ & F1 score $\uparrow$ & & Accuracy $\uparrow$ & F1 score $\uparrow$   \\
\midrule
GIN & 0.496 $\pm$ 0.042 & 0.484 $\pm$ 0.036 & & 0.471 $\pm$ 0.039 & 0482 $\pm$ 0.041 & & 0.537 $\pm$ 0.045 & 0.512  $\pm$ 0.047
\\

GCN & 0.561 $\pm$ 0.049 & 0.535 $\pm$ 0.021 & & 0.520 $\pm$ 0.036 & 0.571 $\pm$ 0.032& & 0.593 $\pm$ 0.039 & 0.561  $\pm$ 0.042 
 \\

\midrule

GIN + GC  & 0.483 $\pm$ 0.026 & 0.472 $\pm$ 0.031 & &  0.486 $\pm$ 0.041 & 0.510 $\pm$ 0.037 & & 0.539 $\pm$ 0.041 & 0.532  $\pm$ 0.069
\\

GCN + GC & 0.522 $\pm$ 0.019 & 0.539 $\pm$ 0.031 & &  0.508 $\pm$ 0.032 & 0.527 $\pm$ 0.031 & & 0.544 $\pm$ 0.025 & 0.582  $\pm$ 0.042
 \\
 
\midrule

GIN + UGC  & 0.561 $\pm$ 0.027 & 0.570 $\pm$ 0.031 & &  0.697 $\pm$ 0.041 & 0.624 $\pm$ 0.037 & & 0.589 $\pm$ 0.041 & 0.562  $\pm$ 0.069
\\

GCN + UGC & 0.572 $\pm$ 0.021 & 0.619 $\pm$ 0.037 & &  0.658 $\pm$ 0.030 & 0.621 $\pm$ 0.021 & & 0.619 $\pm$ 0.025 & 0.581  $\pm$ 0.031
 \\

\midrule
\textbf{UGC-GNN (GIN)} & \textbf{0.624}$\pm$ \textbf{0.036}& \textbf{0.713 }$\pm$ \textbf{0.022} & & \textbf{0.701}$\pm$ \textbf{0.025}& \textbf{0.689}$\pm$ \textbf{0.019} & & \textbf{0.714}$\pm$ \textbf{0.011}& \textbf{0.701}$\pm$ \textbf{0.032}

\\

\textbf{UGC-GNN (GCN)} & \textbf{0.603}$\pm$ \textbf{0.031}& \textbf{0.652 }$\pm$ \textbf{0.020} & & \textbf{0.724}$\pm$ \textbf{0.021}& \textbf{0.697}$\pm$ \textbf{0.019} & & \textbf{0.691}$\pm$ \textbf{0.013}& \textbf{0.706}$\pm$ \textbf{0.029}

\\
\bottomrule
\end{tabular}
}
\end{center}
%\vspace{-10pt}
\caption{Ablation study results. GC = graph canonization, UGC = universal graph canonization. \textbf{Best results} are highlighted.}
\label{tab:abla}
%\vskip -0.16in
\end{table*} 

\textbf{Ablation study reults. Table ~\ref{tab:abla}.} 
This experiment tests the effectiveness of different components in UGC-GNN and empirically supports theoretical findings in the paper. When comparing GIN (GCN), GIN + GC (GCN + GC), and GIN + UGC (GCN + UGC), (1) we find GNNs with general graph canonization usually causes the decrease of the testing performance (i.e. GIN + GC < GIN, GCN + GC < GCN). This finding aligns well with Lemma ~\ref{lemma:2_3}, indicating that stability of GNN is of great practical importance in real datasets especially when graphs are large. (2) We also observe that GNNs with universal graph canonization significantly enhance the model performance, and the observation empirically supports the Lemma ~\ref{lemma:3_4}. Furthermore, we also find that GIN (GCN)< GIN + UGC (GCN + UGC) < and UGC-GNN (GIN or GCN). Consequently, the canonical information from the discrete colouring $\{l(v_1| \mathbb{G}), l(v_2| \mathbb{G}) ... l(v_n| \mathbb{G})\}$ enhance the base GNN architecture from the perspective of both message passing process and the readout function.

\section{Graph Structured Data in Bioinformatics and their GNN Baselines}
\label{sec:appenH}

The dominant graph-structured biological data in bioinformatics can be categorized into three types: (1) molecular graphs, (2) biological interaction graphs and (3) gene networks/graphs. Different types of these biological graph data have different SoTA GNN baselines.
 
In molecular graphs, atoms or other chemical compounds are used as nodes, and the bonds are formulated as the edges. Molecular graphs are homogeneous graphs and are widely used as benchmark datasets in the field of representation learning on graphs and GNNs (graph neural networks). Typical molecular graph benchmark datasets include ZINC, QM9~\cite{ramakrishnan2014quantum}, Molhiv in OGB (Open Graph Benchmark), etc. Dominant baseline deep learning models for these molecular graph datasets are popular GNN models, such as GIN, GCN, GINE, NGNN, PPGN, and these baselines are used in our experimnets.   
 
In biological interaction graphs, nodes represent genes, drugs, disease, RNA, etc, and an edge indicates the existence of a known association between entities connected by the edge.  Thus, biological interaction graphs are heterogeneous graphs. Typical biological interaction graphs include gene-drug interaction networks in the drug synergy prediction task, drug-protein interaction networks ~\cite{zitnik2018modeling} in side effect prediction tasks, and miRNA-disease interaction networks ~\cite{pan2019inferring} in the disease classification task. For the representation learning tasks on biological interaction graphs, various task-specific graph neural networks are proposed, and here we provide some popular examples: TransSynergy ~\cite{liu2021transynergy} and SANEpool ~\cite{dong2023interpreting} for gene-drug interaction networks; Decagon for drug-protein interaction networks; and DimiG ~\cite{pan2019inferring} for miRNA-disease interaction networks. Overall, these task-specific GNNs focus more on how to effectively construct the biological interaction graphs and represent initial features related to genes/drugs/ disease/RNA. Instead of the architecture design of GNNs. Consequently, these task-specific GNNs may not be well generalized to other graph learning tasks such as the gene network representation learning. In the paper, we select TransSynergy, SANEpool, Decagon and DimiG as baselines, and compare them with the proposed UGC-GNN.   
 
In gene graphs/networks, genes are used as nodes, and an edge is used to link two genes if there is a physical signaling interaction between the genes from the documented medical experiment. Similar to molecular graphs, gene graphs/networks are also homogeneous graphs. Very limited works are proposed for gene network representation learning. MLA-GNN is proposed for graph-level classification tasks on gene networks, thus it can be used as a good baseline in the field.
